# Supplementary material for: Origins of anisotropic thermal expansion in flexible materials
Source: arXiv:1707.07705 ancillary file (2017-07-24)
Supplement: Supplementary file 1 [file Supplementary_material.pdf]

# Origins of anisotropic thermal expansion in flexible materials: Supplemental Material

Carl P. Romao

*Department of Chemistry, University of Oxford,*

*Inorganic Chemistry Laboratory, South Parks Road, Oxford OX1 3QR, UK*

(Dated: July 24, 2017)

## I. COMPUTATIONAL PARAMETERS

DFPT calculations of phonon energies and elastic tensors were performed using parameters summarized in Table I. Plane wave (PW) basis set energy cutoffs, Van der Waals (VdW) pairwise tolerances,[1] and **k**-point (electronic) Monkhorst–Pack grid spacings[2] were determined by convergence studies, where the criterion used was convergence within 1 % in the pressure. For zinc and graphite, the **q**-point (phononic) Monkhorst–Pack grids used were subsets of the **k**-point grids due to the fine spacings required for accurate computation of the electronic structures.

TABLE I. Computational parameters determined by convergence studies.

| Material | PW cutoff / Ha | VdW tolerance / Ha | **k**-point grid | **q**-point grid |
|---|---|---|---|---|
| Zinc | 60 | N/A | $24 \times 24 \times 12$ | $6 \times 6 \times 6$ |
| Graphite | 45 | $10^{-11}$ | $16 \times 16 \times 6$ | $8 \times 8 \times 3$ |
| Calcite | 40 | $10^{-10}$ | $6 \times 6 \times 6$ | $6 \times 6 \times 6$ |

## II. ELASTIC TENSORS

### A. Zinc

The stiffness tensor of zinc, as calculated by DFPT, is given by:

$$\boldsymbol{c} = \begin{pmatrix} 204.0 & 31.7 & 30.8 & 0 & 0 & 0 \\ 31.7 & 204.0 & 30.8 & 0 & 0 & 0 \\ 30.8 & 30.8 & 86.9 & 0 & 0 & 0 \\ 0 & 0 & 0 & 42.4 & 0 & 0 \\ 0 & 0 & 0 & 0 & 42.4 & 0 \\ 0 & 0 & 0 & 0 & 0 & 86.2 \end{pmatrix} \times \text{GPa}. \tag{1}$$

Comparison to experimental results (Ref. 3) reveals that the calculated bulk modulus (75 GPa) is in reasonable agreement with the experimental result at 0 K (80 GPa), although there are discrepancies for some elements of the tensor.

### B. Graphite

The stiffness tensor of graphite, as calculated by DFPT, is given by:

$$\boldsymbol{c} = \begin{pmatrix} 1090.7 & 195.9 & -10.7 & 0 & 0 & 0 \\ 195.9 & 1090.7 & -10.7 & 0 & 0 & 0 \\ -10.7 & -10.7 & 45.0 & 0 & 0 & 0 \\ 0 & 0 & 0 & 6.4 & 0 & 0 \\ 0 & 0 & 0 & 0 & 6.4 & 0 \\ 0 & 0 & 0 & 0 & 0 & 447.4 \end{pmatrix} \times \text{GPa}. \tag{2}$$

The calculated bulk modulus (40 GPa) is essentially identical to the experimental result at 0 K (40 GPa), and in general the calculated tensor is close to the experimental one.[4]

### C. Calcite

The stiffness tensor of calcite, as calculated by DFPT, is given by:

$$\boldsymbol{c} = \begin{pmatrix} 160.7 & 65.0 & 58.6 & 0 & 21.7 & 0 \\ 65.0 & 160.7 & 58.6 & 0 & -21.7 & 0 \\ 58.6 & 58.6 & 82.3 & 0 & 0 & 0 \\ 0 & 0 & 0 & 33.5 & 0 & -21.7 \\ 21.7 & -21.7 & 0 & 0 & 33.5 & 0 \\ 0 & 0 & 0 & -21.7 & 0 & 47.8 \end{pmatrix} \times \text{GPa}. \tag{3}$$

The calculated bulk modulus (75 GPa) is extremely close to the experimental result at 0 K (76 GPa), and in general the calculated tensor is calculated tensor is close to the experimental one.[5]

## III. MODE GRÜNEISEN PARAMETERS

Phonon energies and mode Grüneisen parameters of zinc and graphite calculated by DFPT are shown in Figs. 1 and 2.

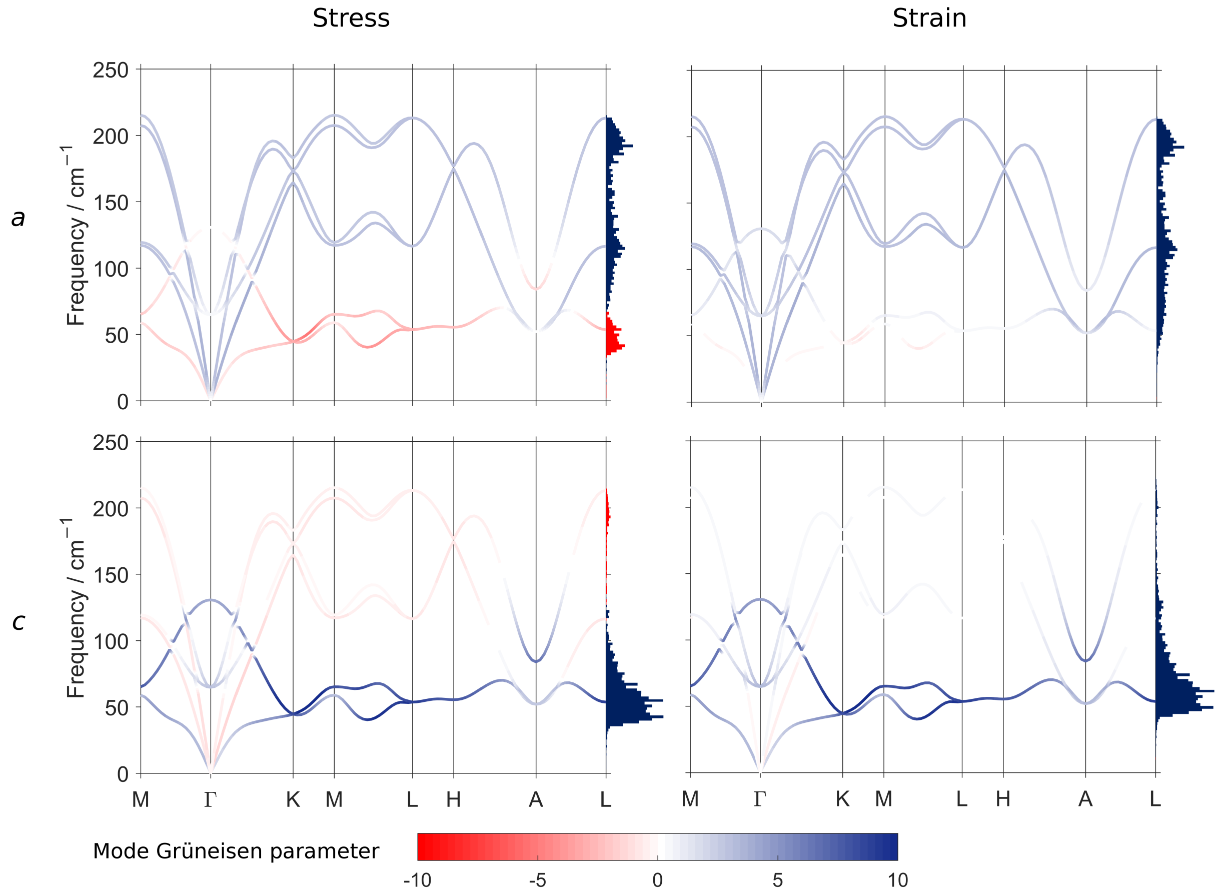


FIG. 1. Phonon band structure of zinc, with bands coloured according to their axial mode Grüneisen parameters calculated using stress and strain perturbations. The density of states ($\rho$), weighted by the Grüneisen parameters as $\sum_{\mathbf{k}} \rho_{\mathbf{k}}(\omega)\gamma_{n,\mathbf{k}}(\omega)$, is shown as a histogram at the right of each plot, with positive values coloured in blue and negative values in red. Special points in and paths through the Brillouin zone were selected following Ref. 6.

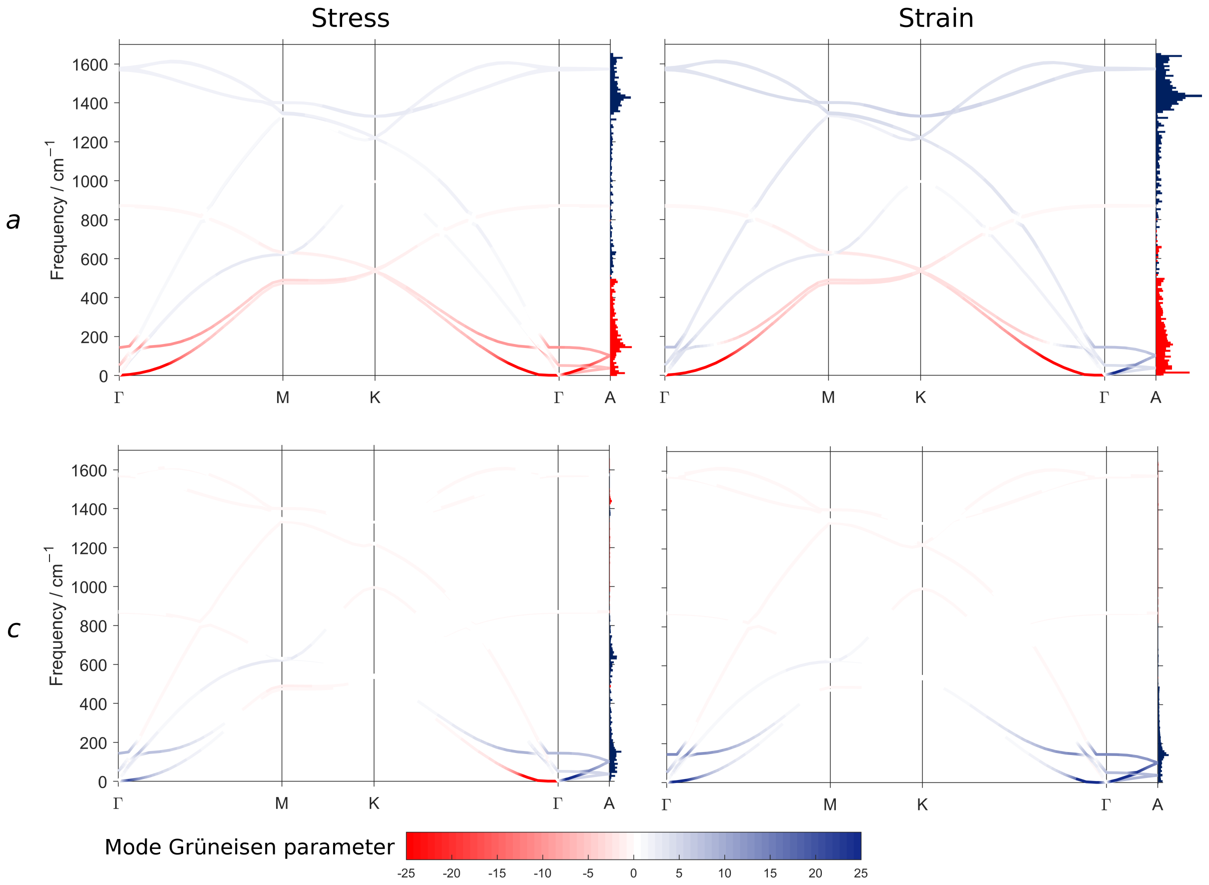


FIG. 2. Phonon band structure of graphite, with bands coloured according to their axial mode Grüneisen parameters calculated using stress and strain perturbations. The density of states ($\rho$), weighted by the Grüneisen parameters as $\sum_{\mathbf{k}} \rho_{\mathbf{k}}(\omega)\gamma_{n,\mathbf{k}}(\omega)$, is shown as a histogram at the right of each plot, with positive values coloured in blue and negative values in red. Special points in and paths through the Brillouin zone were selected following Ref. 6.

[1] B. Van Troeye, M. Torrent, and X. Gonze, Phys. Rev. B **93**, 144304 (2016).

[2] H. J. Monkhorst and J. D. Pack, Phys. Rev. B **13**, 5188 (1976).

[3] H. M. Ledbetter, J. Phys. Chem. Ref. Data **6**, 1181 (1977).

[4] W. B. Gauster and I. J. Fritz, **45**, 3309 (1974).

[5] D. P. Dandekar and A. L. Ruoff, Journal of Applied Physics **39**, 6004 (1968).

[6] W. Setyawan and S. Curtarolo, **49**, 299 (2010).
